# Supplementary material for: Optical Manipulation of Domains in Chiral Topological Superconductors
Source: arXiv:2010.00838 source file (2020-12-16)
Supplement: Supplementary file 1 [file Supplemental_Material.pdf]

# Optical Manipulation of Domains in Chiral Topological Superconductors: Supplemental Material


Tao Yu,[1] Martin Claassen,[2,3] Dante M. Kennes,[4] and Michael A. Sentef[1]

[1] *Max Planck Institute for the Structure and Dynamics of Matter, Luruper Chaussee 149, 22761 Hamburg, Germany*

[2] *Center for Computational Quantum Physics, Simons Foundation Flatiron Institute, New York, NY, USA*

[3] *Department of Physics, University of Pennsylvania, Philadelphia, PA 19104, USA*

[4] *Institut für Theorie der Statistischen Physik, RWTH Aachen, 52056 Aachen, Germany*



(Dated: October 2, 2020)

# I. EFFECTIVE LAGRANGIAN

We start the derivation from the $t$-$J$ model Hamiltonian of the honeycomb lattice (Fig. S1) [1–4]

$$\hat{H}_{t-J} = -t \sum_{\langle i,j\rangle,\sigma} \hat{a}^{\dagger}_{i\sigma}\hat{b}_{j\sigma} + \text{H.c.} - \mu \sum_{i,\sigma}(\hat{a}^{\dagger}_{i\sigma}\hat{a}_{i\sigma} + \hat{b}^{\dagger}_{i\sigma}\hat{b}_{i\sigma}) - J\sum_{\langle i,j\rangle} \hat{h}^{\dagger}_{ij}\hat{h}_{ij}, \tag{S1}$$

where $\hat{h}^{\dagger}_{ij} = (\hat{a}^{\dagger}_{i\uparrow}\hat{b}^{\dagger}_{j\downarrow} - \hat{a}^{\dagger}_{i\downarrow}\hat{b}^{\dagger}_{j\uparrow})$. The parameters and operators are introduced in the main text. Based on the

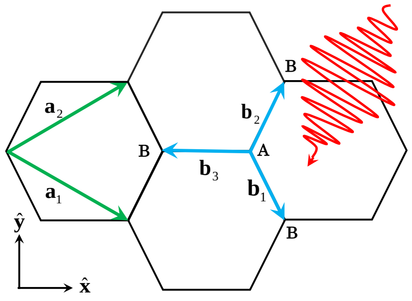


FIG. S1. Optical engineering of chiral superconductivity on a honeycomb lattice. Geometrical parameters are indicated: $\mathbf{b}_{\mu=1,2,3}$ are three bonding vectors connecting B and A lattices, which define the two primitive vectors of the lattice by $\mathbf{a}_1 = \mathbf{b}_1 - \mathbf{b}_3$ and $\mathbf{a}_2 = \mathbf{b}_2 - \mathbf{b}_3$. An in-plane optical driving is applied as indicated by the red arrow.

lattice model, we define the continuous field operators

$$\hat{\psi}_A(\mathbf{r}) = \frac{1}{\sqrt{S}}\sum_{\mathbf{k}} \hat{a}(\mathbf{k})e^{i\mathbf{k}\cdot\mathbf{r}}, \quad \hat{\psi}_B(\mathbf{r}) = \frac{1}{\sqrt{S}}\sum_{\mathbf{k}} \hat{b}(\mathbf{k})e^{i\mathbf{k}\cdot\mathbf{r}},$$

where $S = N\Omega$ is the area of $N$ unit cells with $\Omega = \sqrt{3}a^2/2 = 3\sqrt{3}b^2/2$ being the area of one unit cell. Here, $a = |\mathbf{a}_1| = |\mathbf{a}_2|$ and $b = |\mathbf{b}_{\mu=\{1,2,3\}}|$, introduced in Fig. S1. The anticommutation relations $\left\{\hat{\psi}^{\dagger}_i(\mathbf{r}), \hat{\psi}_j(\mathbf{r}')\right\} = \delta(\mathbf{r}-\mathbf{r}')\delta_{ij}$ are guaranteed. In terms of the field operator $\hat{\Psi}(\mathbf{r}) = \left(\hat{\psi}_{A\uparrow}(\mathbf{r}), \hat{\psi}_{B\uparrow}(\mathbf{r}), \hat{\psi}^{\dagger}_{A\downarrow}(\mathbf{r}), \hat{\psi}^{\dagger}_{B\downarrow}(\mathbf{r})\right)^T$ in the Nambu space, the free part of the Hamiltonian is written as

$$\hat{H}_0 = \int d\mathbf{r}\hat{\Psi}^{\dagger}(\mathbf{r}) \begin{pmatrix} -\mu & -tf(\hat{\mathbf{k}}) & 0 & 0 \\ -tf^{\dagger}(\hat{\mathbf{k}}) & -\mu & 0 & 0 \\ 0 & 0 & \mu & tf^{\dagger}(-\hat{\mathbf{k}}) \\ 0 & 0 & tf(-\hat{\mathbf{k}}) & \mu \end{pmatrix} \hat{\Psi}(\mathbf{r}), \tag{S2}$$

where $f(\mathbf{k}) = \sum_{\mu} e^{i\mathbf{k}\cdot\mathbf{b}_{\mu}}$, while the interaction Hamiltonian is

$$\hat{H}_{\text{int}} = -J\Omega\sum_{\mu}\int d\mathbf{r}\left(\hat{\Psi}^{\dagger}(\mathbf{r}_{\mu})\tau_A\hat{\Psi}(\mathbf{r}) + \hat{\Psi}^{\dagger}(\mathbf{r})\tau_B\hat{\Psi}(\mathbf{r}_{\mu})\right)\left(\hat{\Psi}^{\dagger}(\mathbf{r})\tau_A^T\hat{\Psi}(\mathbf{r}_{\mu}) + \hat{\Psi}^{\dagger}(\mathbf{r}_{\mu})\tau_B^T\hat{\Psi}(\mathbf{r})\right), \tag{S3}$$

with $\mathbf{r}_{\mu} = \mathbf{r} + \mathbf{b}_{\mu}$, $\tau_A = \begin{pmatrix} 0&0&0&0 \\ 0&0&1&0 \\ 0&0&0&0 \\ 0&0&0&0 \end{pmatrix}$, and $\tau_B = \begin{pmatrix} 0&0&0&1 \\ 0&0&0&0 \\ 0&0&0&0 \\ 0&0&0&0 \end{pmatrix}$.

Accordingly, with the Grassmann field $\overline{\Psi}(\mathbf{r},\tau) = \left(\overline{\psi}_{A\uparrow}(\mathbf{r}), \overline{\psi}_{B\uparrow}(\mathbf{r}), \psi_{A\downarrow}(\mathbf{r}), \psi_{B\downarrow}(\mathbf{r})\right)$, the action reads

$$\begin{aligned}\mathcal{S} &= \int_0^\beta d\tau d\mathbf{r}\overline{\Psi}(\mathbf{r},\tau)\partial_\tau\Psi(\mathbf{r},\tau) + \int_0^\beta d\tau d\mathbf{r}\overline{\Psi}(\mathbf{r},\tau)H_0(\hat{\mathbf{k}})\Psi(\mathbf{r},\tau) \\ &- J\Omega\sum_\mu\int_0^\beta d\tau d\mathbf{r}\left(\overline{\Psi}(\mathbf{r}_\mu)\tau_A\Psi(\mathbf{r}) + \overline{\Psi}(\mathbf{r})\tau_B\Psi(\mathbf{r}_\mu)\right)\left(\overline{\Psi}(\mathbf{r})\tau_A^T\Psi(\mathbf{r}_\mu) + \overline{\Psi}(\mathbf{r}_\mu)\tau_B^T\Psi(\mathbf{r})\right). \end{aligned} \tag{S4}$$

The Grassmann field is periodic with $\Psi(\tau = 0) = \Psi(\tau = \beta)$ and $\overline{\Psi}(\tau = 0) = -\overline{\Psi}(\tau = \beta)$. We introduce the complex Bose fields $\phi(\mathbf{r},\mathbf{r}_\mu)$ by Hubbard-Stratonovich transformation [5]

$$1 = \int\mathcal{D}\phi(\mathbf{r},\mathbf{r}_\mu)\mathcal{D}\overline{\phi}(\mathbf{r},\mathbf{r}_\mu)\exp\left(-\int_0^\beta d\tau\sum_\mu\int d\mathbf{r}\overline{\phi}(\mathbf{r},\mathbf{r}_\mu)\frac{1}{J\Omega}\phi(\mathbf{r},\mathbf{r}_\mu)\right).$$

A shift of the Bose field $\phi(\mathbf{r},\mathbf{r}_\mu) \to \phi(\mathbf{r},\mathbf{r}_\mu) + J\Omega\left(\overline{\Psi}(\mathbf{r},\tau)\tau_A^T\Psi(\mathbf{r}_\mu,\tau) + \overline{\Psi}(\mathbf{r}_\mu,\tau)\tau_B^T\Psi(\mathbf{r},\tau)\right)$ yields the action

$$\begin{aligned}\mathcal{S}_{\text{pair}} &= \int_0^\beta d\tau d\mathbf{r}\overline{\Psi}(\mathbf{r},\tau)\partial_\tau\Psi(\mathbf{r},\tau) + \int_0^\beta d\tau d\mathbf{r}\overline{\Psi}(\mathbf{r},\tau)H_0(\hat{\mathbf{k}})\Psi(\mathbf{r},\tau) \\ &+ \sum_\mu\int_0^\beta d\tau d\mathbf{r}\overline{\phi}(\mathbf{r},\mathbf{r}_\mu)\frac{1}{J\Omega}\phi(\mathbf{r},\mathbf{r}_\mu) \\ &+ \sum_\mu\int_0^\beta d\tau d\mathbf{r}\overline{\phi}(\mathbf{r},\mathbf{r}_\mu)\left(\overline{\Psi}(\mathbf{r})\tau_A^T\Psi(\mathbf{r}_\mu) + \overline{\Psi}(\mathbf{r}_\mu)\tau_B^T\Psi(\mathbf{r})\right) \\ &+ \sum_\mu\int_0^\beta d\tau d\mathbf{r}\left(\overline{\Psi}(\mathbf{r}_\mu)\tau_A\Psi(\mathbf{r}) + \overline{\Psi}(\mathbf{r})\tau_B\Psi(\mathbf{r}_\mu)\right)\phi(\mathbf{r},\mathbf{r}_\mu). \end{aligned} \tag{S5}$$

The fermion singlets, in the last two terms, can mediate an effective interaction between the order parameters $\phi(\mathbf{r},\mathbf{r}_\mu)$ after being integrated out. To perform this integration, we go to the momentum-frequency space for the fermion Grassmann field

$$\Psi(\tau,\mathbf{r}) = \frac{1}{\sqrt{\beta}}\frac{1}{\sqrt{S}}\sum_{\mathbf{k}}\sum_{\omega_n}\Psi(\omega_n,\mathbf{k})e^{-i\omega_n\tau}e^{i\mathbf{k}\cdot\mathbf{r}}, \tag{S6}$$

and for the boson field with respect to the *center-of-mass* coordinate $\mathbf{r} + \mathbf{r}_\mu/2$

$$\phi(\tau,\mathbf{r},\mathbf{r}+\mathbf{b}_\mu) = \frac{1}{\sqrt{\beta}}\frac{1}{\sqrt{S}}\sum_{\mathbf{k}}\sum_{\omega_m}\phi(\omega_m,\mathbf{k})e^{-i\omega_n\tau}e^{i\mathbf{k}\cdot(\mathbf{r}+\mathbf{b}_\mu/2)}. \tag{S7}$$

With $k \equiv \{\omega_n,\mathbf{k}\}$ and $q \equiv \{\omega_m,\mathbf{q}\}$, we arrive at the partition function

$$Z = \int\mathcal{D}\overline{\phi}_\mu(q)\mathcal{D}\phi_\mu(q)\exp\left(-\mathcal{S}_{\text{eff}}[\overline{\phi},\phi]\right),$$

with an effective action for the boson field,

$$\mathcal{S}_{\text{eff}}[\overline{\phi},\phi] = \sum_\mu\sum_q\overline{\phi}_\mu(q)\frac{1}{J\Omega}\phi_\mu(q) - \operatorname{tr}\ln\left(-\hat{G}^{-1}(\phi,\overline{\phi})\right). \tag{S8}$$

Here, $\operatorname{tr}(...) = \sum_k\langle k|...|k\rangle$, $\hat{G}^{-1}[\phi] = i\hat{\omega} - \hat{H}_0 - \hat{\Phi}$, in which the matrix elements of operators read

$$\begin{aligned}\langle k|\hat{\Phi}|k'\rangle &= \frac{1}{\sqrt{\beta S}}\sum_\mu\left(\overline{\phi}_\mu(k'-k)\left(e^{i\boldsymbol{\mathcal{K}}\cdot\mathbf{b}_\mu}\tau_A^T + e^{-i\boldsymbol{\mathcal{K}}\cdot\mathbf{b}_\mu}\tau_B^T\right) + \phi_\mu(k-k')\left(e^{-i\boldsymbol{\mathcal{K}}\cdot\mathbf{b}_\mu}\tau_A + e^{i\boldsymbol{\mathcal{K}}\cdot\mathbf{b}_\mu}\tau_B\right)\right), \\ \langle k|(-i\hat{\omega} + \hat{H}_0)|k'\rangle &= (-i\omega_n + \hat{H}_0(\mathbf{k}))\delta_{kk'} \end{aligned} \tag{S9}$$

with $\boldsymbol{\kappa} = (\mathbf{k}+\mathbf{k}')/2$ denoting the center-of-mass momentum. When the order parameter is small, it can be used to expand the action,

$$\mathcal{S}_{\text{eff}}[\overline{\phi},\phi] = \sum_{\mu}\sum_{q}\overline{\phi}_{\mu}(q)\frac{1}{J\Omega}\phi_{\mu}(q) + \frac{1}{2}\sum_{kk'}\text{tr}\left(G^0_k\Phi_{k,k'}G^0_{k'}\Phi_{k',k}\right) + \frac{1}{S}\int d\mathbf{r}\frac{1}{4}\sum_{k}\text{tr}\left(G_{0k}\Phi_{\mathbf{k}}G_{0k}\Phi_{\mathbf{k}}G_{0k}\Phi_{\mathbf{k}}G_{0k}\Phi_{\mathbf{k}}\right), \tag{S10}$$

where the first two terms are linear while the third term is nonlinear.

## A. Linear term

From the first two terms in Eq. (S10), we arrive at the linear effective action

$$\mathcal{S}^L_{\text{eff}}[\overline{\phi},\phi] = \sum_{\mu q}\overline{\phi}_{\mu}(q)\frac{1}{J\Omega}\phi_{\mu}(q) + \frac{1}{\beta}\frac{1}{S}\sum_{kq}\sum_{\mu\mu'}B^{\mu\mu'}_{k-\frac{q}{2},k+\frac{q}{2}}\overline{\phi}_{\mu}(q)\phi_{\mu'}(q), \tag{S11}$$

where

$$B^{\mu\mu'}_{k-\frac{q}{2},k+\frac{q}{2}} = \text{tr}\left(G^0_{k-\frac{q}{2}}(e^{i\mathbf{k}\cdot\mathbf{b}_{\mu}}\tau^T_A + e^{-i\mathbf{k}\cdot\mathbf{b}_{\mu}}\tau^T_B)G^0_{k+\frac{q}{2}}(e^{-i\mathbf{k}\cdot\mathbf{b}_{\mu'}}\tau_A + e^{i\mathbf{k}\cdot\mathbf{b}_{\mu'}}\tau_B)\right). \tag{S12}$$

Here, $G_0(\omega_m,\mathbf{k}) = \text{diag}\{G_e(\omega_m,\mathbf{k}), G_h(\omega_m,\mathbf{k})\}$ is the Green function of the free Hamiltonian in the Nambu space, where the Green functions in the electron and hole space read

$$\begin{aligned} G_e(\mathbf{k},\omega_m) &= \frac{P_1(\mathbf{k})}{i\omega_m - \varepsilon_1(\mathbf{k})} + \frac{P_2(\mathbf{k})}{i\omega_m - \varepsilon_2(\mathbf{k})}, \\ G_h(\mathbf{k},\omega_m) &= \frac{P_1(\mathbf{k})}{i\omega_m + \varepsilon_1(\mathbf{k})} + \frac{P_2(\mathbf{k})}{i\omega_m + \varepsilon_2(\mathbf{k})}. \end{aligned} \tag{S13}$$

Here, $\varepsilon_1(\mathbf{k}) = t|f(\mathbf{k})| - \mu$ and $\varepsilon_2(\mathbf{k}) = -t|f(\mathbf{k})| - \mu$ are the electron and hole dispersions, and

$$P_1(\mathbf{k}) = \frac{1}{2}\begin{pmatrix} 1 & -e^{i\phi_{\mathbf{k}}} \\ -e^{-i\phi_{\mathbf{k}}} & 1 \end{pmatrix}, \quad P_2(\mathbf{k}) = \frac{1}{2}\begin{pmatrix} 1 & e^{i\phi_{\mathbf{k}}} \\ e^{-i\phi_{\mathbf{k}}} & 1 \end{pmatrix} \tag{S14}$$

are the projection operators for the two bands. With Green function Eq. (S13), we obtain

$$\begin{aligned} B^{\mu\mu'}_{k-\frac{q}{2},k+\frac{q}{2}} &= \frac{1}{2}\left(\frac{1}{i\omega_m + \varepsilon_1(\mathbf{k}-\frac{\mathbf{q}}{2})}\frac{1}{i\omega_m - \varepsilon_1(\mathbf{k}+\frac{\mathbf{q}}{2})} + \frac{1}{i\omega_m + \varepsilon_2(\mathbf{k}-\frac{\mathbf{q}}{2})}\frac{1}{i\omega_m - \varepsilon_2(\mathbf{k}+\frac{\mathbf{q}}{2})}\right) \\ &\times\left(\cos\left[\mathbf{k}\cdot(\mathbf{b}_{\mu}+\mathbf{b}_{\mu'}) - \varphi_{\mathbf{k}-\frac{\mathbf{q}}{2}} - \varphi_{\mathbf{k}+\frac{\mathbf{q}}{2}}\right] + \cos\mathbf{k}\cdot(\mathbf{b}_{\mu}-\mathbf{b}_{\mu'})\right) \\ &+ \frac{1}{2}\left(\frac{1}{i\omega_m + \varepsilon_1(\mathbf{k}-\frac{\mathbf{q}}{2})}\frac{1}{i\omega_m - \varepsilon_2(\mathbf{k}+\frac{\mathbf{q}}{2})} + \frac{1}{i\omega_m + \varepsilon_2(\mathbf{k}-\frac{\mathbf{q}}{2})}\frac{1}{i\omega_m - \varepsilon_1(\mathbf{k}+\frac{\mathbf{q}}{2})}\right) \\ &\times\left(-\cos\left[\mathbf{k}\cdot(\mathbf{b}_{\mu}+\mathbf{b}_{\mu'}) - \varphi_{\mathbf{k}-\frac{\mathbf{q}}{2}} - \varphi_{\mathbf{k}+\frac{\mathbf{q}}{2}}\right] + \cos\mathbf{k}\cdot(\mathbf{b}_{\mu}-\mathbf{b}_{\mu'})\right), \end{aligned} \tag{S15}$$

which is an even function of $\mathbf{q}$. Assuming a small $\mathbf{q}$, we define the mass and fluctuation terms

$$\begin{aligned} &\frac{1}{S}\frac{1}{\beta}\sum_{k}B^{\mu\mu'}_{k,k} + \frac{1}{J\Omega}\delta_{\mu\mu'} \equiv \mathcal{M}^{\mu\mu'}(q=0), \\ &\frac{1}{S}\frac{1}{\beta}\sum_{k}\left(B^{\mu\mu'}_{k-q/2,k+q/2} - B^{\mu\mu'}_{k,k}\right)\Big|_{\omega_q\to0,\mathbf{q}\to0} \longrightarrow \sum_{\delta\gamma}\mathcal{T}^{\mu\mu'}_{\delta\gamma}\mathbf{q}_{\delta}\mathbf{q}_{\gamma}. \end{aligned} \tag{S16}$$

Thus, the fluctuation of long range is determined by

$$\mathcal{T}^{\mu\mu'}_{\delta\gamma} \equiv \begin{pmatrix} T^{11} & T^{12} & T^{13} \\ T^{12} & T^{22} & T^{23} \\ T^{13} & T^{23} & T^{33} \end{pmatrix}_{\delta\gamma} = \frac{1}{2}\frac{\partial^2}{\partial\mathbf{q}_{\delta}\partial\mathbf{q}_{\gamma}}\left(\frac{1}{S}\frac{1}{\beta}\sum_{k}B^{\mu\mu'}_{k-\frac{q}{2},k+\frac{q}{2}}\right)\Big|_{\omega_q\to0,\mathbf{q}\to0}, \tag{S17}$$

where we calculate the summation over momentum and Matsubara frequency

$$
\begin{aligned}
\mathcal{B}_{\mathbf{q}}^{\mu\mu'} &\equiv \frac{1}{S}\frac{1}{\beta}\sum_{k} B^{\mu\mu'}_{k-\frac{q}{2},k+\frac{q}{2}} \\
&= \frac{1}{2S}\sum_{\mathbf{k}}\left(\frac{n_F\left(\varepsilon_1(\mathbf{k}-\frac{\mathbf{q}}{2})\right)+n_F(\varepsilon_1\left(\mathbf{k}+\frac{\mathbf{q}}{2}\right))-1}{\varepsilon_1\left(\mathbf{k}-\frac{\mathbf{q}}{2}\right)+\varepsilon_1\left(\mathbf{k}+\frac{\mathbf{q}}{2}\right)}+\frac{n_F\left(\varepsilon_2(\mathbf{k}-\frac{\mathbf{q}}{2})\right)+n_F(\varepsilon_2\left(\mathbf{k}+\frac{\mathbf{q}}{2}\right))-1}{\varepsilon_2\left(\mathbf{k}-\frac{\mathbf{q}}{2}\right)+\varepsilon_2\left(\mathbf{k}+\frac{\mathbf{q}}{2}\right)}\right) \\
&\times\left(\cos\left(\mathbf{k}\cdot(\mathbf{b}_\mu+\mathbf{b}_{\mu'})-\phi_{\mathbf{k}-\frac{\mathbf{q}}{2}}-\phi_{\mathbf{k}+\frac{\mathbf{q}}{2}}\right)+\cos\mathbf{k}\cdot(\mathbf{b}_\mu-\mathbf{b}_{\mu'})\right) \\
&+\frac{1}{2S}\sum_{\mathbf{k}}\left(\frac{n_F\left(\varepsilon_1(\mathbf{k}-\frac{\mathbf{q}}{2})\right)+n_F(\varepsilon_2\left(\mathbf{k}+\frac{\mathbf{q}}{2}\right))-1}{\varepsilon_1\left(\mathbf{k}-\frac{\mathbf{q}}{2}\right)+\varepsilon_2\left(\mathbf{k}+\frac{\mathbf{q}}{2}\right)}+\frac{n_F\left(\varepsilon_2(\mathbf{k}-\frac{\mathbf{q}}{2})\right)+n_F(\varepsilon_1\left(\mathbf{k}+\frac{\mathbf{q}}{2}\right))-1}{\varepsilon_2\left(\mathbf{k}-\frac{\mathbf{q}}{2}\right)+\varepsilon_1\left(\mathbf{k}+\frac{\mathbf{q}}{2}\right)}\right) \\
&\times\left(-\cos\left(\mathbf{k}\cdot(\mathbf{b}_\mu+\mathbf{b}_{\mu'})-\phi_{\mathbf{k}-\frac{\mathbf{q}}{2}}-\phi_{\mathbf{k}+\frac{\mathbf{q}}{2}}\right)+\cos\mathbf{k}\cdot(\mathbf{b}_\mu-\mathbf{b}_{\mu'})\right). \qquad \text{(S18)}
\end{aligned}
$$

The inverse Fourier transformation $\phi_\mu(q)=\frac{1}{\sqrt{S}}\frac{1}{\sqrt{\beta}}\int d\tau d\mathbf{r} e^{i\omega_m\tau}e^{-i\mathbf{q}\cdot(\mathbf{r}+\mathbf{b}_\mu/2)}\phi_\mu(\tau,\mathbf{r})$ can bring the action back to the time-spatial space, yielding the effective action

$$
\mathcal{S}^L_{\text{eff}}[\overline{\phi},\phi]=\sum_{\mu\mu'}\int_0^\beta d\tau d\mathbf{r}\overline{\phi}_\mu(\mathbf{r},\tau)\mathcal{M}^{\mu\mu'}\phi_{\mu'}(\mathbf{r},\tau)+\sum_{\mu\mu'}\sum_{\delta\gamma}\mathcal{T}^{\mu\mu'}_{\delta\gamma}\int_0^\beta d\tau d\mathbf{r}\partial_\delta\phi^*_\mu(\mathbf{r},\tau)\partial_\gamma\phi_{\mu'}(\mathbf{r},\tau). \qquad \text{(S19)}
$$

The gap equation is given by the saddle point solution $\delta S_{\text{eff}}(\overline{\phi},\phi)/\delta\overline{\phi}_q\Big|_{q\to 0}=0$, leading to the eigenvalue equation for the vector fields $\vec{\Phi}=(\phi_1,\phi_2,\phi_3)^T$,

$$
\frac{1}{J\Omega}\vec{\Phi}=\begin{pmatrix}\mathcal{A} & \mathcal{B} & \mathcal{B}\\ \mathcal{B} & \mathcal{A} & \mathcal{B}\\ \mathcal{B} & \mathcal{B} & \mathcal{A}\end{pmatrix}\vec{\Phi}, \qquad \text{(S20)}
$$

where $\mathcal{A}=-\mathcal{B}^{\mu\mu}_{\mathbf{q}=0}$ and $\mathcal{B}=-\mathcal{B}^{\mu\mu'}_{\mathbf{q}=0}|_{\mu\neq\mu'}$. The first eigenvalue $1/J=\Omega(\mathcal{A}+2\mathcal{B})$ corresponds to the extended $s$-wave state with eigenvector $\vec{\Delta}_s=(1,1,1)^T/\sqrt{3}$, and the remaining two eigenvalues $1/J=\Omega(\mathcal{A}-\mathcal{B})$ are degenerate, corresponding to the $d$-wave order parameters with two degenerate eigenvectors

$$
\begin{aligned}
\vec{\Delta}_a &= \frac{1}{\sqrt{6}}(2,-1,-1)^T, \qquad d_{x^2-y^2}, \\
\vec{\Delta}_b &= \frac{1}{\sqrt{2}}(0,1,-1)^T, \qquad d_{xy}. \qquad \text{(S21)}
\end{aligned}
$$

The superposition of $\vec{\Delta}_a$ and $\vec{\Delta}_b$ gives different types of $d$-wave superconductivity. Particularly, superposition $\frac{\sqrt{2}}{2}\left(\vec{\Delta}_a+i\vec{\Delta}_b\right)=\frac{1}{\sqrt{3}}\left(1,e^{i\frac{2\pi}{3}},e^{i\frac{4\pi}{3}}\right)^T$ gives the $d_{x^2-y^2}+id_{xy}$ wave, while $\frac{\sqrt{2}}{2}\left(\vec{\Delta}_a-i\vec{\Delta}_b\right)=\frac{1}{\sqrt{3}}\left(1,e^{i\frac{4\pi}{3}},e^{i\frac{2\pi}{3}}\right)^T$ gives the $d_{x^2-y^2}-id_{xy}$ wave. We decompose $\phi_\mu$ by the new basis with

$$
\Phi(\mathbf{r},t)=(\phi_1(\mathbf{r},t),\phi_2(\mathbf{r},t),\phi_3(\mathbf{r},t))^T=\eta_1(\mathbf{r},t)\xi_1+\eta_2(\mathbf{r},t)\xi_2+\eta_3(\mathbf{r},t)\xi_3, \qquad \text{(S22)}
$$

where $\xi_1=\frac{1}{\sqrt{3}}\left(1,e^{i2\pi/3},e^{i4\pi/3}\right)^T$, $\xi_2=\frac{1}{\sqrt{3}}\left(1,e^{i4\pi/3},e^{i2\pi/3}\right)^T$ and $\xi_3=\frac{1}{\sqrt{3}}(1,1,1)^T$ are the basis for the order parameters in $(d_{x^2-y^2}+id_{xy})$-wave, $(d_{x^2-y^2}-id_{xy})$-wave and $s$-wave, respectively, and $\eta_i$ denote the amplitudes of these order parameters.

In terms of order-parameter amplitudes $\eta_i(\mathbf{r})$, we express the linear Ginzburg-Landau (GL) Lagrangian as

$$
\begin{aligned}
L_{\text{eff}} &= \sum_{i=\{1,2,3\}}(\xi_i^\dagger\boldsymbol{\mathcal{M}}\xi_i)\int d\mathbf{r}\eta_i^*(\mathbf{r})\eta_i(\mathbf{r})+\sum_{\delta\gamma}\sum_{ij}(\xi_i^\dagger\boldsymbol{\mathcal{T}}_{\delta\gamma}\xi_j)\int d\mathbf{r}\partial_\delta\eta_i^*(\mathbf{r})\partial_\gamma\eta_j(\mathbf{r}) \\
&= \sum_i a_i\int d\mathbf{r}\eta_i^*(\mathbf{r})\eta_i(\mathbf{r})+\sum_{\delta\gamma}\sum_{ij}c^{ij}_{\delta\gamma}\int d\mathbf{r}\partial_\delta\eta_i^*(\mathbf{r})\partial_\gamma\eta_j(\mathbf{r}), \qquad \text{(S23)}
\end{aligned}
$$

where the coefficients $a_i \equiv \xi_i^\dagger \boldsymbol{\mathcal{M}} \xi_i$ and $c_{\delta\gamma}^{ij} \equiv \xi_i^\dagger \boldsymbol{\mathcal{T}}_{\delta\gamma} \xi_j$ are governed by symmetry and band structure. These coefficients are simply parameterized by several real quantities $\{a, a', b, b', e_1, e_2\}$. For $a_i$, $a_1 = a_2 = a$ and $a_3 = a'$, following the gap equation near $T_c$. When $i = j = \{1, 2, 3\}$,

$$c_{\delta\gamma}^{11} = c_{\delta\gamma}^{22} = b\delta_{\delta\gamma}, \quad c_{\delta\gamma}^{33} = b'\delta_{\delta\gamma};$$

when $i \neq j$, we find

$$\begin{aligned} c_{xx}^{21} &= e_1(1 - i\sqrt{3}), \quad c_{yy}^{21} = -e_1(1 - i\sqrt{3}), \quad c_{xy}^{21} = c_{yx}^{21} = ie_1(1 - i\sqrt{3}), \\ c_{xx}^{31} &= e_2(1 + i\sqrt{3}), \quad c_{yy}^{31} = -e_2(1 + i\sqrt{3}), \quad c_{xy}^{31} = c_{yx}^{31} = -ie_2(1 + i\sqrt{3}), \\ c_{xx}^{32} &= e_2(1 - i\sqrt{3}), \quad c_{yy}^{32} = -e_2(1 - i\sqrt{3}), \quad c_{xy}^{32} = c_{yx}^{32} = ie_2(1 - i\sqrt{3}), \end{aligned}$$

and $c_{\delta\gamma}^{ji} = (c_{\delta\gamma}^{ij})^*$ that guarantees the Hermiticity. These analysis simplifies the linear GL Lagrangian to be

$$\begin{aligned} L_{\text{eff}} = &\, a \int d\mathbf{r} \left( |\eta_1(\mathbf{r})|^2 + |\eta_2(\mathbf{r})|^2 \right) + a' \int d\mathbf{r} |\eta_3(\mathbf{r})|^2 \\ &+ b \int d\mathbf{r} \left( |\partial_x \eta_1(\mathbf{r})|^2 + |\partial_y \eta_1(\mathbf{r})|^2 + |\partial_x \eta_2(\mathbf{r})|^2 + |\partial_y \eta_2(\mathbf{r})|^2 \right) \\ &+ b' \int d\mathbf{r} \left( |\partial_x \eta_3(\mathbf{r})|^2 + |\partial_y \eta_3(\mathbf{r})|^2 \right) \\ &+ e_1(1 - i\sqrt{3}) \int d\mathbf{r} (\partial_x + i\partial_y)\eta_2^*(\mathbf{r})(\partial_x + i\partial_y)\eta_1(\mathbf{r}) + \text{h.c.} \\ &+ e_2(1 + i\sqrt{3}) \int d\mathbf{r} (\partial_x - i\partial_y)\eta_3^*(\mathbf{r})(\partial_x - i\partial_y)\eta_1(\mathbf{r}) + \text{h.c.} \\ &+ e_2(1 - i\sqrt{3}) \int d\mathbf{r} (\partial_x + i\partial_y)\eta_3^*(\mathbf{r})(\partial_x + i\partial_y)\eta_2(\mathbf{r}) + \text{h.c.}, \end{aligned} \tag{S24}$$

where the coefficients with different chemical potentials are numerically calculated in this work. The form of the gradient terms can be simply understood from the angular momentum conservation. The system has $C_6$ symmetry, given by operators, e.g., $\hat{C}_6^1 = e^{i\frac{2\pi}{6}J_z}$. Since $\partial_x + i\partial_y$ and $\partial_x - i\partial_y$ have angular momentum $+1$ and $-1$, while $\eta_1$, $\eta_2$ and $\eta_3$ have angular momentum $+2$, $-2$ and 0, the total angular momentum of every gradient term has to be the interger times of 6. For example, term $\int d\mathbf{r}(\partial_x + i\partial_y)\eta_2^*(\mathbf{r})(\partial_x + i\partial_y)\eta_1(\mathbf{r})$ has angular momentum 6.

### B. Nonlinear terms

For the derivation of the nonlinear term, we can treat the order parameter to be homogeneous by

$$\phi_\mu(\mathbf{k} = 0) = \frac{1}{\sqrt{S}} \int d\mathbf{r} \phi_\mu(\mathbf{r}) \approx \sqrt{S}\phi_\mu(\mathbf{r}). \tag{S25}$$

With $\Phi_{\mathbf{k}} = \frac{1}{\sqrt{\beta}} \sum_\mu \left( \bar{\phi}_\mu Q_\mu^T(\mathbf{k}) + \phi_\mu Q_\mu(-\mathbf{k}) \right)$ where $Q_\mu^T(\mathbf{k}) = e^{i\mathbf{k}\cdot\mathbf{b}_\mu}\tau_A^T + e^{-i\mathbf{k}\cdot\mathbf{b}_\mu}\tau_B^T$, the dominant nonlinear term in the Lagrangian reads

$$\begin{aligned} L_{\text{eff}}^{\text{NL}} = &\frac{1}{S} \int d\mathbf{r} \frac{1}{4\beta^2} \sum_{\mu_1\mu_2\mu_3\mu_4} \text{tr} \Big[ G_{0k}(\bar{\phi}_{\mu_1} Q_{\mu_1}^T(\mathbf{k}) + \phi_{\mu_1} Q_{\mu_1}(-\mathbf{k})) G_{0k}(\bar{\phi}_{\mu_2} Q_{\mu_2}^T(\mathbf{k}) + \phi_{\mu_2} Q_{\mu_2}(-\mathbf{k})) \\ &\times G_{0k}(\bar{\phi}_{\mu_3} Q_{\mu_3}^T(\mathbf{k}) + \phi_{\mu_3} Q_{\mu_3}(-\mathbf{k})) G_{0k}(\bar{\phi}_{\mu_4} Q_{\mu_4}^T(\mathbf{k}) + \phi_{\mu_4} Q_{\mu_4}(-\mathbf{k})) \Big]. \end{aligned} \tag{S26}$$

Although with complicated form, it is simplified by using

$$Q^T_{\mu_i} = \begin{pmatrix} 0 & 0 \\ \square^T_{\mu_i} & 0 \end{pmatrix}, \quad Q_{\mu_i} = \begin{pmatrix} 0 & \square_{\mu_i} \\ 0 & 0 \end{pmatrix}, \tag{S27}$$

and the Green function in the subspace

$$G_{0k}Q^T_{\mu_i} = \begin{pmatrix} 0 & 0 \\ G^h_k\square^T_{\mu_i} & 0 \end{pmatrix}, \quad G_{0k}Q_{\mu_i} = \begin{pmatrix} 0 & G^e_k\square_{\mu_i} \\ 0 & 0 \end{pmatrix}, \tag{S28}$$

since $G_{0k}Q^T_{\mu_i}G_{0k}Q^T_{\mu_j} = 0$. The nonlinear term is reduced to

$$L^{\mathrm{NL}}_{\mathrm{eff}} = \frac{1}{S}\int d\mathbf{r}\frac{1}{2\beta^2}\sum_k\sum_{\mu_i}\bar{\phi}_{\mu_1}\phi_{\mu_2}\bar{\phi}_{\mu_3}\phi_{\mu_4}\mathrm{tr}\Big[G^h_k\square^T_{\mu_1}(\mathbf{k})G^e_k\square_{\mu_2}(-\mathbf{k})G^h_k\square^T_{\mu_3}(\mathbf{k})G^e_k\square_{\mu_4}(-\mathbf{k})\Big]. \tag{S29}$$

With relation $\square_\mu(-\mathbf{k}) = \square^T_\mu(\mathbf{k}) = \begin{pmatrix} 0 & e^{i\mathbf{k}\cdot\mathbf{b}_\mu} \\ e^{-i\mathbf{k}\cdot\mathbf{b}_\mu} & 0 \end{pmatrix}$ in mind, we obtain

$$L^{\mathrm{NL}}_{\mathrm{eff}} = \frac{1}{S}\int d\mathbf{r}\frac{1}{2\beta^2}\sum_k\sum_{\mu_i}\bar{\phi}_{\mu_1}\phi_{\mu_2}\bar{\phi}_{\mu_3}\phi_{\mu_4}\mathrm{tr}\Big[G_{0k}Q^T_{\mu_1}(\mathbf{k})G_{0k}Q_{\mu_2}(-\mathbf{k})G_{0k}Q^T_{\mu_3}(\mathbf{k})G_{0k}Q_{\mu_4}(-\mathbf{k})\Big]. \tag{S30}$$

Focusing on the $d$-waves, we have the bonding order parameter

$$\begin{aligned} \phi_1 &= \frac{1}{\sqrt{3}}(\eta_1 + \eta_2), \\ \phi_2 &= \frac{1}{\sqrt{3}}(\eta_1 e^{i2\pi/3} + \eta_2 e^{i4\pi/3}), \\ \phi_3 &= \frac{1}{\sqrt{3}}(\eta_1 e^{i4\pi/3} + \eta_2 e^{i2\pi/3}), \end{aligned} \tag{S31}$$

and $\sum_\mu \bar{\phi}_\mu(\mathbf{k})\Lambda_\mu(\mathbf{k}) = \eta_1^*\Lambda_1(\mathbf{k}) + \eta_2^*\Lambda_2(\mathbf{k})$ with

$$\begin{aligned} \Lambda_1(\mathbf{k}) &= \frac{1}{\sqrt{3}}\begin{pmatrix} 0 & e^{i\mathbf{k}\cdot\mathbf{b}_1} + e^{i\frac{4\pi}{3}}e^{i\mathbf{k}\cdot\mathbf{b}_2} + e^{i\frac{2\pi}{3}}e^{i\mathbf{k}\cdot\mathbf{b}_3} \\ e^{-i\mathbf{k}\cdot\mathbf{b}_1} + e^{i\frac{4\pi}{3}}e^{-i\mathbf{k}\cdot\mathbf{b}_2} + e^{i\frac{2\pi}{3}}e^{-i\mathbf{k}\cdot\mathbf{b}_3} & 0 \end{pmatrix}, \\ \Lambda_2(\mathbf{k}) &= \frac{1}{\sqrt{3}}\begin{pmatrix} 0 & e^{i\mathbf{k}\cdot\mathbf{b}_1} + e^{i\frac{2\pi}{3}}e^{i\mathbf{k}\cdot\mathbf{b}_2} + e^{i\frac{4\pi}{3}}e^{i\mathbf{k}\cdot\mathbf{b}_3} \\ e^{-i\mathbf{k}\cdot\mathbf{b}_1} + e^{i\frac{2\pi}{3}}e^{-i\mathbf{k}\cdot\mathbf{b}_2} + e^{i\frac{4\pi}{3}}e^{-i\mathbf{k}\cdot\mathbf{b}_3} & 0 \end{pmatrix}. \end{aligned} \tag{S32}$$

We see $\Lambda_2^*(-\mathbf{k}) = \Lambda_1(\mathbf{k})$ or $\Lambda_1^*(-\mathbf{k}) = \Lambda_2(\mathbf{k})$. The nonlinear part in the Lagrangian then becomes

$$\begin{aligned} L^{\mathrm{NL}}_{\mathrm{eff}} = \frac{1}{S}\int d\mathbf{r}\frac{1}{2\beta^2}\sum_k \mathrm{tr}\Big[&G^h_k(\eta_1^*(\mathbf{r})\Lambda_1(\mathbf{k}) + \eta_2^*(\mathbf{r})\Lambda_2(\mathbf{k}))G^e_k(\eta_1(\mathbf{r})\Lambda_2(\mathbf{k}) + \eta_2(\mathbf{r})\Lambda_1(\mathbf{k})) \\ &\times G^h_k(\eta_1^*(\mathbf{r})\Lambda_1(\mathbf{k}) + \eta_2^*(\mathbf{r})\Lambda_2(\mathbf{k}))G^e_k(\eta_1(\mathbf{r})\Lambda_2(\mathbf{k}) + \eta_2(\mathbf{r})\Lambda_1(\mathbf{k}))\Big]. \end{aligned} \tag{S33}$$

There are still many terms that should be further simplified. We can generally demonstrate that only the terms with two $\Lambda_1(\mathbf{k})$ and $\Lambda_2(\mathbf{k})$ can survive among them by the $C_3$ symmetry of the system, dramatically simplifying the calculations. With using $C_3^{-1}\mathbf{k}\cdot\mathbf{b}_\mu = \mathbf{k}\cdot C_3\mathbf{b}_\mu$, we know that a $C_3$ operation gives a transformation $\{\mathbf{b}_1, \mathbf{b}_2, \mathbf{b}_3\} \to \{\mathbf{b}_2, \mathbf{b}_3, \mathbf{b}_1\}$. Such a transformation then leads to

$$\Lambda_1(\mathbf{k}) \to e^{-i2\pi/3}\Lambda_1(\mathbf{k}), \quad \Lambda_2(\mathbf{k}) \to e^{i2\pi/3}\Lambda_2(\mathbf{k}). \tag{S34}$$

This transformation gives $C \to e^{\pm i2\pi/3}C = 0$ apart from the terms with two $\Lambda_1(\mathbf{k})$ and $\Lambda_2(\mathbf{k})$. We write down all these (six) terms and analyze their property in a general way:

$$\begin{aligned}
① &= \frac{1}{2\beta^2}\frac{1}{S}\sum_k \mathrm{tr}\left[G_k^h\Lambda_1(\mathbf{k})G_k^e\Lambda_2(\mathbf{k})G_k^h\Lambda_1(\mathbf{k})G_k^e\Lambda_2(\mathbf{k})\right] \to |\eta_1(\mathbf{r})|^4 \\
② &= \frac{1}{2\beta^2}\frac{1}{S}\sum_k \mathrm{tr}\left[G_k^h\Lambda_2(\mathbf{k})G_k^e\Lambda_1(\mathbf{k})G_k^h\Lambda_2(\mathbf{k})G_k^e\Lambda_1(\mathbf{k})\right] \to |\eta_2(\mathbf{r})|^4 \\
③ &= \frac{1}{2\beta^2}\frac{1}{S}\sum_k \mathrm{tr}\left[G_k^h\Lambda_1(\mathbf{k})G_k^e\Lambda_1(\mathbf{k})G_k^h\Lambda_2(\mathbf{k})G_k^e\Lambda_2(\mathbf{k})\right] \to |\eta_1(\mathbf{r})|^2|\eta_2(\mathbf{r})|^2 \\
④ &= \frac{1}{2\beta^2}\frac{1}{S}\sum_k \mathrm{tr}\left[G_k^h\Lambda_2(\mathbf{k})G_k^e\Lambda_2(\mathbf{k})G_k^h\Lambda_1(\mathbf{k})G_k^e\Lambda_1(\mathbf{k})\right] \to |\eta_1(\mathbf{r})|^2|\eta_2(\mathbf{r})|^2 \\
⑤ &= \frac{1}{2\beta^2}\frac{1}{S}\sum_k \mathrm{tr}\left[G_k^h\Lambda_1(\mathbf{k})G_k^e\Lambda_2(\mathbf{k})G_k^h\Lambda_2(\mathbf{k})G_k^e\Lambda_1(\mathbf{k})\right] \to |\eta_1(\mathbf{r})|^2|\eta_2(\mathbf{r})|^2 \\
⑥ &= \frac{1}{2\beta^2}\frac{1}{S}\sum_k \mathrm{tr}\left[G_k^h\Lambda_2(\mathbf{k})G_k^e\Lambda_1(\mathbf{k})G_k^h\Lambda_1(\mathbf{k})G_k^e\Lambda_2(\mathbf{k})\right] \to |\eta_1(\mathbf{r})|^2|\eta_2(\mathbf{r})|^2.
\end{aligned} \tag{S35}$$

We domonstrate below that these terms can gather to two coefficients in terms of $f_1$ and $f_2$.

We can demonstrate that ① = ②. We note that $G_h(\mathbf{k}, -\omega_m) = -G_e(\mathbf{k}, \omega_m)$, leading to

$$\begin{aligned}
② &= \frac{1}{2\beta^2}\frac{1}{S}\sum_{\mathbf{k}}\sum_{\omega_m} \mathrm{tr}\left[G_h(\mathbf{k},-\omega_m)\Lambda_2(\mathbf{k})G_e(\mathbf{k},-\omega_m)\Lambda_1(\mathbf{k})G_h(\mathbf{k},-\omega_m)\Lambda_2(\mathbf{k})G_e(\mathbf{k},-\omega_m)\Lambda_1(\mathbf{k})\right] \\
&= \frac{1}{2\beta^2}\frac{1}{S}\sum_{\mathbf{k}}\sum_{\omega_m} \mathrm{tr}\left[G_e(\mathbf{k},\omega_m)\Lambda_2(\mathbf{k})G_h(\mathbf{k},\omega_m)\Lambda_1(\mathbf{k})G_e(\mathbf{k},\omega_m)\Lambda_2(\mathbf{k})G_h(\mathbf{k},\omega_m)\Lambda_1(\mathbf{k})\right] \\
&= \frac{1}{2\beta^2}\frac{1}{S}\sum_{\mathbf{k}}\sum_{\omega_m} \mathrm{tr}\left[G_h(\mathbf{k},\omega_m)\Lambda_1(\mathbf{k})G_e(\mathbf{k},\omega_m)\Lambda_2(\mathbf{k})G_h(\mathbf{k},\omega_m)\Lambda_1(\mathbf{k})G_e(\mathbf{k},\omega_m)\Lambda_2(\mathbf{k})\right] = ①.
\end{aligned}$$

We can also show the two terms are real: We note that the Green function also satisfies $G_h^*(-\mathbf{k}, \omega_m) = -G_e(\mathbf{k}, \omega_m)$ or $G_e^*(-\mathbf{k}, \omega_m) = -G_h(\mathbf{k}, \omega_m)$. By taking the conjugation and using $\mathbf{k} \to -\mathbf{k}$,

$$\begin{aligned}
②^* &= \frac{1}{2\beta^2}\frac{1}{S}\sum_{\mathbf{k}}\sum_{\omega_m} \mathrm{tr}\left[G_h^*(-\mathbf{k},\omega_m)\Lambda_2^*(-\mathbf{k})G_e^*(-\mathbf{k},\omega_m)\Lambda_1^*(-\mathbf{k})G_h^*(-\mathbf{k},\omega_m)\Lambda_2^*(-\mathbf{k})G_e^*(-\mathbf{k},\omega_m)\Lambda_1^*(-\mathbf{k})\right] \\
&= \frac{1}{2\beta^2}\frac{1}{S}\sum_{\mathbf{k}}\sum_{\omega_m} \mathrm{tr}\left[G_e(\mathbf{k},\omega_m)\Lambda_1(\mathbf{k})G_h(\mathbf{k},\omega_m)\Lambda_2(\mathbf{k})G_e(\mathbf{k},\omega_m)\Lambda_1(\mathbf{k})G_h(\mathbf{k},\omega_m)\Lambda_2(\mathbf{k})\right] \\
&= \frac{1}{2\beta^2}\frac{1}{S}\sum_{\mathbf{k}}\sum_{\omega_m} \mathrm{tr}\left[G_h(\mathbf{k},\omega_m)\Lambda_2(\mathbf{k})G_e(\mathbf{k},\omega_m)\Lambda_1(\mathbf{k})G_h(\mathbf{k},\omega_m)\Lambda_2(\mathbf{k})G_e(\mathbf{k},\omega_m)\Lambda_1(\mathbf{k})\right] = ②.
\end{aligned}$$

We define ① = ② = $f_1 + f_2$. On the other hand, it is similar to demonstrate ③ = ④ and ⑤ = ⑥. We can also demonstrate that ③ and ⑤ are real, e.g.,

$$\begin{aligned}
⑤^* &= \frac{1}{2\beta^2}\frac{1}{S}\sum_{\mathbf{k}}\sum_{\omega_m} \mathrm{tr}\left[G_h^*(-\mathbf{k},\omega_m)\Lambda_1^*(-\mathbf{k})G_e^*(-\mathbf{k},\omega_m)\Lambda_2^*(-\mathbf{k})G_h^*(-\mathbf{k},\omega_m)\Lambda_2^*(-\mathbf{k})G_e^*(-\mathbf{k},\omega_m)\Lambda_1^*(-\mathbf{k})\right] \\
&= \frac{1}{2\beta^2}\frac{1}{S}\sum_{\mathbf{k}}\sum_{\omega_m} \mathrm{tr}\left[G_e(\mathbf{k},\omega_m)\Lambda_2(\mathbf{k})G_h(\mathbf{k},\omega_m)\Lambda_1(\mathbf{k})G_e(\mathbf{k},\omega_m)\Lambda_1(\mathbf{k})G_h(\mathbf{k},\omega_m)\Lambda_2(\mathbf{k})\right] \\
&= \frac{1}{2\beta^2}\frac{1}{S}\sum_{\mathbf{k}}\sum_{\omega_m} \mathrm{tr}\left[G_e(\mathbf{k},-\omega_m)\Lambda_1(\mathbf{k})G_h(\mathbf{k},-\omega_m)\Lambda_2(\mathbf{k})G_e(\mathbf{k},-\omega_m)\Lambda_2(\mathbf{k})G_h(\mathbf{k},-\omega_m)\Lambda_1(\mathbf{k})\right] \\
&= \frac{1}{2\beta^2}\frac{1}{S}\sum_{\mathbf{k}}\sum_{\omega_m} \mathrm{tr}\left[G_h(\mathbf{k},\omega_m)\Lambda_1(\mathbf{k})G_e(\mathbf{k},\omega_m)\Lambda_2(\mathbf{k})G_h(\mathbf{k},\omega_m)\Lambda_2(\mathbf{k})G_e(\mathbf{k},\omega_m)\Lambda_1(\mathbf{k})\right] = ⑤.
\end{aligned}$$

When we write ③ + ⑤ = $f_1 - f_2$, the nonlinear part of the GL Lagrangian reads

$$L_{\mathrm{eff}}^{\mathrm{NL}} = \int d\mathbf{r}\left(f_1\left(|\eta_1|^2 + |\eta_2|^2\right)^2 + f_2\left(|\eta_1|^2 - |\eta_2|^2\right)^2\right). \tag{S36}$$

We now can work out the concrete value of $f_1$ and $f_2$. We have

$$
\begin{aligned}
f_1+f_2 &= \frac{1}{2\beta^2}\frac{1}{S}\sum_k \mathrm{tr}\left[G^h_k\Lambda_1(\mathbf{k})G^e_k\Lambda_2(\mathbf{k})G^h_k\Lambda_1(\mathbf{k})G^e_k\Lambda_2(\mathbf{k})\right],\\
f_1-f_2 &= \frac{1}{2\beta^2}\frac{1}{S}\sum_k \mathrm{tr}\left[G^h_k\Lambda_1(\mathbf{k})G^e_k\Lambda_1(\mathbf{k})G^h_k\Lambda_2(\mathbf{k})G^e_k\Lambda_2(\mathbf{k})\right]\\
&\quad+\frac{1}{2\beta^2}\frac{1}{S}\sum_k \mathrm{tr}\left[G^h_k\Lambda_1(\mathbf{k})G^e_k\Lambda_2(\mathbf{k})G^h_k\Lambda_2(\mathbf{k})G^e_k\Lambda_1(\mathbf{k})\right].
\end{aligned}
\tag{S37}
$$

We restrict to a high electron doping, in which case the electron and hole Green functions are approximated by $G^h_k \approx \frac{P_1(\mathbf{k})}{i\omega_m+\varepsilon_1(\mathbf{k})}$ and $G^e_k \approx \frac{P_1(\mathbf{k})}{i\omega_m-\varepsilon_1(\mathbf{k})}$, with which, e.g.,

$$
f_1+f_2 \simeq \frac{1}{2\beta^2}\frac{1}{S}\sum_{\mathbf{k}}\sum_{\omega_m}\mathrm{tr}\left[\frac{P_1(\mathbf{k})\Lambda_1(\mathbf{k})P_1(\mathbf{k})\Lambda_2(\mathbf{k})P_1(\mathbf{k})\Lambda_1(\mathbf{k})P_1(\mathbf{k})\Lambda_2(\mathbf{k})}{(i\omega_m+\varepsilon_1(\mathbf{k}))^2(i\omega_m-\varepsilon_1(\mathbf{k}))^2}\right].
$$

We calculate the integral according to the residue theorem and arrive at

$$
\begin{aligned}
f_1+f_2 &= \frac{1}{2\beta}\frac{1}{S}\sum_{\mathbf{k}}\mathrm{tr}\left[P_1(\mathbf{k})\Lambda_1(\mathbf{k})P_1(\mathbf{k})\Lambda_2(\mathbf{k})P_1(\mathbf{k})\Lambda_1(\mathbf{k})P_1(\mathbf{k})\Lambda_2(\mathbf{k})\right]\\
&\quad\times\left[\frac{1}{4\varepsilon_1^2(\mathbf{k})}\Big(n'_F(\varepsilon_1(\mathbf{k}))+n'_F(-\varepsilon_1(\mathbf{k}))\Big)+\frac{1}{4\varepsilon_1^3(\mathbf{k})}\Big(-n_F(\varepsilon_1(\mathbf{k}))+n_F(-\varepsilon_1(\mathbf{k}))\Big)\right],
\end{aligned}
\tag{S38}
$$

where $n_F(z)=1/(e^{\beta z}+1)$. A similar expression is obtained for $f_1-f_2$.

## II. TIME-DEPENDENT GINZBURG-LANDAU EQUATION

We first use GL Lagrangian to analyze the equilibrium state, in which we also include the static magnetic field. According to the gauge invariance, we incorporate the magnetic field into the Lagrangian by adding the vector potential with substitution $\nabla-\frac{2e}{i\hbar c}\mathbf{A}(\mathbf{r})$ for $\eta$ term, where $c$ is the light velocity and $\mathbf{A}$ is the vector potential of the *static* magnetic field. The Lagrangian *density* for the $d$-wave order parameter is written by

$$
\begin{aligned}
\mathcal{L}_{\text{eff}}(\mathbf{r}) &= a\sum_{\mu=1,2}|\eta_\mu(\mathbf{r})|^2\\
&\quad+b\sum_{\nu=x,y}\sum_{\mu}\left(\partial_\nu+\frac{2e}{i\hbar c}\mathbf{A}_\nu(\mathbf{r})\right)\eta^*_\mu(\mathbf{r})\left(\partial_\nu-\frac{2e}{i\hbar c}\mathbf{A}_\nu(\mathbf{r})\right)\eta_\mu(\mathbf{r})\\
&\quad+e_1(1-i\sqrt{3})\left(\partial_+-\frac{2e}{i\hbar c}\mathbf{A}_+(\mathbf{r})\right)\eta^*_2(\mathbf{r})\left(\partial_+-\frac{2e}{i\hbar c}\mathbf{A}_+(\mathbf{r})\right)\eta_1(\mathbf{r})\\
&\quad+e_1(1+i\sqrt{3})\left(\partial_-+\frac{2e}{i\hbar c}\mathbf{A}_-(\mathbf{r})\right)\eta_2(\mathbf{r})\left(\partial_-+\frac{2e}{i\hbar c}\mathbf{A}_-(\mathbf{r})\right)\eta^*_1(\mathbf{r})\\
&\quad+f_1\left(|\eta_1(\mathbf{r})|^2+|\eta_2(\mathbf{r})|^2\right)^2+f_2\left(|\eta_1(\mathbf{r})|^2-|\eta_2(\mathbf{r})|^2\right)^2,
\end{aligned}
\tag{S39}
$$

where $\partial_\pm=\partial_x\pm i\partial_y$ and $\mathbf{A}_\pm=\mathbf{A}_x\pm i\mathbf{A}_y$. We have disregarded the $s$-wave order parameter in the Lagrangian density since $a'>0$, by our calculation, indicates that the $s$-wave superconductivity is not energetically favored. We estimate the parameters by using $t=2.7$ eV, $J=0.25t$ and $|\mathbf{b}|=2.46/\sqrt{3}$ Å for the single layer graphene. For the chemical potentials $\mu/t=\{0.85,0.9,0.95,1,1.05,1.1\}$, the critical temperature is calculated to be $T_c=\{1.23,4.74,19.18,40.05,15.98,2.95\}$ K, exhibiting a dome around the doping with $\mu=t$. Above or below this region, the superconductivity no longer exist. Increasing $J$ may exponentially increase $T_c$. We note that $e_1$ approaches zero when $\mu\to t$ and becomes opposite with $\mu>t$ and $\mu<t$. We then choose

$T = 1.5$ K and dopings with $\mu/t = \{0.9, 1.1\}$ as the typical cases to illustrate the chirality switch dynamics. We summarize the calculated parameters in Table I.

TABLE I. Calculated coefficients for single layer graphene superconductivity. In the table, $t = 2.7$ eV and $|\mathbf{b}| = 2.46/\sqrt{3} \times 10^{-10}$ for the graphene. The units of the parameters are $\{a, a'\} \to \text{meV}^{-1} \cdot \text{m}^{-2}$, $\{b, b', e_1, e_2\} \to \text{meV}^{-1}$, $\{f_1, f_2\} \to \text{meV}^{-3} \cdot \text{m}^{-2}$.

| $\mu/t$ | $a/(10^{-4})$ | $a'/(10^{-4})$ | $b$ | $b'$ | $e_1$ | $e_2$ | $f_1$ | $f_2$ |
|---|---|---|---|---|---|---|---|---|
| 0.9 | $-9.97/\lvert\mathbf{b}\rvert^2$ | $3.0/\lvert\mathbf{b}\rvert^2$ | 800.4 | 530.3 | 150.2 | 100.0 | $2.1/\lvert\mathbf{b}\rvert^2$ | $-0.7/\lvert\mathbf{b}\rvert^2$ |
| 1.1 | $-4.12/\lvert\mathbf{b}\rvert^2$ | $1.8/\lvert\mathbf{b}\rvert^2$ | 1631.6 | 1048.1 | $-109.3$ | 270.3 | $1.9/\lvert\mathbf{b}\rvert^2$ | $-0.6/\lvert\mathbf{b}\rvert^2$ |

Without the external field, we may expect that the order parameter is homogeneous to minimize the free energy density. We can demonstrate that $\{|\eta_1|, |\eta_2|\} = \eta_0\{1, 0\}$ and $\eta_0\{0, 1\}$ are two degenerate states that minimize the free energy density. To this end,

$$\begin{aligned}\frac{\partial \mathcal{L}_{\text{eff}}}{\partial|\eta_1|} &= 2a|\eta_1| + 4f_1\left(|\eta_1|^2 + |\eta_2|^2\right)|\eta_1| + 4f_2(|\eta_1|^2 - |\eta_2|^2)|\eta_1| = 0,\\ \frac{\partial \mathcal{L}_{\text{eff}}}{\partial|\eta_2|} &= 2a|\eta_2| + 4f_1\left(|\eta_1|^2 + |\eta_2|^2\right)|\eta_2| - 4f_2(|\eta_1|^2 - |\eta_2|^2)|\eta_2| = 0.\end{aligned} \tag{S40}$$

The solutions gives local minimus are degenerate:

$$\begin{aligned}&①,\quad |\eta_1| = 0,\quad |\eta_2| = \sqrt{-\frac{a}{2(f_1+f_2)}} \equiv \eta_0,\\ &②,\quad |\eta_2| = 0,\quad |\eta_1| = \sqrt{-\frac{a}{2(f_1+f_2)}}.\end{aligned} \tag{S41}$$

The superconductivity is spontaneously broken to one of the two classes. In Fig. S2(a), with parameters of $\mu = 0.9t$ in Table I, the profile of the free energy is plotted with respect to $|\eta_1|$ and $|\eta_2|$, in which we calculate $\eta_0 = 0.02$ meV that identifies the minimum of free energy. The free energy is normalized by $f_0 = 10^{11}$ eV/nm$^2$. In Fig. S2(b), we calculate and plot the additional free energy $\delta f$ of the chirality domain wall in the one dimensional case. We see the surface energy of the domain wall is positive and hence the domain is metastable. With our parameters, the wall width is about 1 $\mu$m.

A laser field may cause interesting dynamics of the $d \pm id$ superconductivity. To this end, we construct the Time-Dependent Ginzburg Landau equation by adding the time-dependent term of the Gross-Pitaevski and Klein-Gordon types and obtain the Lagrangian *density* [6]

$$\begin{aligned}\mathcal{L}_{\text{eff}}(\mathbf{r}) =& \sum_{\mu=1,2}\Gamma_\mu \eta_\mu^*(\mathbf{r})\left(\partial_t - \frac{2e}{i\hbar}\varphi(\mathbf{r})\right)\eta_\mu(\mathbf{r}) + \sum_{\mu=1,2}\Lambda_\mu\left|\left(\partial_t - \frac{2e}{i\hbar}\varphi(\mathbf{r})\right)\eta_\mu(\mathbf{r})\right|^2\\ &+ a\sum_\mu \eta_\mu^*(\mathbf{r})\eta_\mu(\mathbf{r}) + b\sum_{\nu=x,y}\sum_\mu\left(\partial_\nu + \frac{2e}{i\hbar c}\mathbf{A}_\nu(\mathbf{r})\right)\eta_\mu^*(\mathbf{r})\left(\partial_\nu - \frac{2e}{i\hbar c}\mathbf{A}_\nu(\mathbf{r})\right)\eta_\mu(\mathbf{r})\\ &+ e_1(1 - i\sqrt{3})\left(\partial_+ - \frac{2e}{i\hbar c}\mathbf{A}_+(\mathbf{r})\right)\eta_2^*(\mathbf{r})\left(\partial_+ - \frac{2e}{i\hbar c}\mathbf{A}_+(\mathbf{r})\right)\eta_1(\mathbf{r})\\ &+ e_1(1 + i\sqrt{3})\left(\partial_- + \frac{2e}{i\hbar c}\mathbf{A}_-(\mathbf{r})\right)\eta_2(\mathbf{r})\left(\partial_- + \frac{2e}{i\hbar c}\mathbf{A}_-(\mathbf{r})\right)\eta_1^*(\mathbf{r})\\ &+ f_1\left[\eta_1^*(\mathbf{r})\eta_1(\mathbf{r}) + \eta_2^*(\mathbf{r})\eta_2(\mathbf{r})\right]^2 + f_2\left[\eta_1^*(\mathbf{r})\eta_1(\mathbf{r}) - \eta_2^*(\mathbf{r})\eta_2(\mathbf{r})\right]^2,\end{aligned} \tag{S42}$$

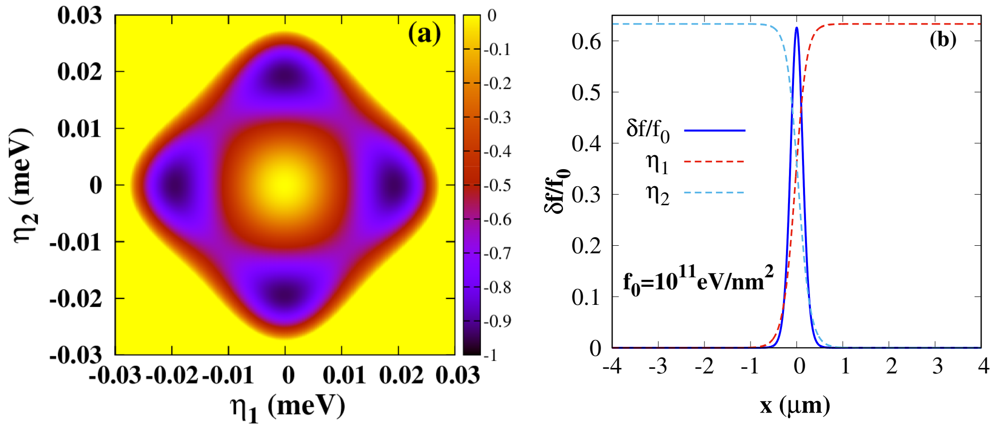


FIG. S2. (Color online) Free energy density of the chiral superconductor. In (a), the free energy density with respect to the different values of $\eta_1$ and $\eta_2$ is plotted, in which the minimum represents the ground state of the superconductor. In (b), we plot the additional free energy $\delta f$ of the chirality domain wall in the one dimensional case.

where $\varphi(\mathbf{r})$ is the scalar potential and $\Gamma$ accounts for the damping of the order parameter to its equilibrium value [6], and $\Lambda$-term is related to the Higgs mode excitation [7]. The further analysis of this Lagrangian is given in the main text.

Here we only address the erasure of chiral domain, which is essential for application, since the combination of creation and annihilation can move a chiral domain on demand, potentially allowing for the braiding of Majorana modes. On the basis of the chiral domain in Fig. 3(b) and (c) of the main text, we now apply similar optical pulses but use the left-circularly polarized laser that favors the switching from $\eta_2$ to $\eta_1$. In Fig. S3 we show the erasure of the chiral domain. The diffusion of order parameters at the edge leaves a ring of chiral domain with a small size, which, however, can be erased by pulses of larger size, such as $\sigma_r = 90$ $\mu$m, shown in Fig. S3(b).

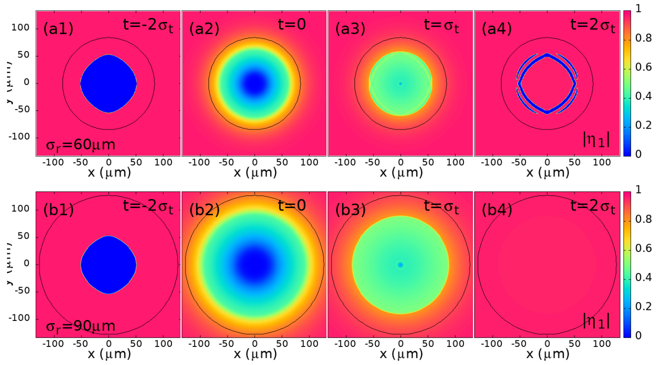


FIG. S3. Optical erasure of a chiral domain (normalized by $\eta_0$) in real space by laser spots of different sizes $\sigma_r = 60$ $\mu$m (a1-a4) and $\sigma_r = 90$ $\mu$m (b1-b4). The spot sizes $\sqrt{2}\sigma_r$ are indicated by black circles. The second pulse is left-circularly polarized and favors the switching from $\eta_2$ to $\eta_1$, as shown by the snapshots (a4) and (b4).

## III. IMPLEMENTING HADAMARD GATES USING MAJORANA EDGE MODES

The ability to optically control the topography of chiral superconducting domains provides a handle to implement quantum operations via braiding of Majorana modes. Here, the key idea is a straightforward extension of recent proposal [8] that exploits the domain wall modes at interfaces between $p{+}ip$ superconductors and quantum anomalous Hall insulators, whose edges carry single Majorana and single complex fermions (which can equivalently be represented as pairs of Majorana fermions), respectively. To translate this idea to optically-controlled $p + ip$ chiral superconductors, note that domain walls between $p + ip$ and $p - ip$ chiral domains similiarly carry *two* Majorana modes, and hence act in analogy to the edge states of a quantum anomalous Hall insulator, depicted in Fig. 1 in the main text.

In this scheme, presume that two metallic leads are patterned over two domain walls between $p + ip/p - ip$ domains, as shown in Fig. 1 of the main text. The single-electron charging states $|0\rangle$, $|1\rangle$ of the two leads now define two single-qubit states: as one injects single electrons into the leads, these propagate chirally along the domain wall boundary until they reach the sample edge (or equivalently, an interface with a trivial insulator). At this point, the complex fermion edge mode fractionalizes into two Majorana modes, which entails a fractionalization of the injected electron. As each Majorana fermion proceeds to travel along the boundary mode and completes a revolution around the circuit, one can see that for the left-side circuit in Fig. 1 two of the Majorana fermions that originate from an electron injected into the left-side and right-side lead are exchanged. If the left-side and right-side charging states are represented via Majorana operators

$$\begin{aligned} \hat{c}_L &: \hat{\gamma}_L^1, \hat{\gamma}_L^2, \\ \hat{c}_R &: \hat{\gamma}_R^1, \hat{\gamma}_R^2, \end{aligned} \tag{S43}$$

respectively, the resulting braiding operation follows from an exchange

$$\begin{aligned} \hat{\gamma}_L^2 &\to \hat{\gamma}_R^2, \\ \hat{\gamma}_R^2 &\to -\hat{\gamma}_L^2. \end{aligned} \tag{S44}$$

Expressed in charging basis, this exchange implements a non-Abelian operation. For instance, if the initial charging states take the form $|1\rangle\,|0\rangle$, then the braiding operation transforms this to

$$|1\rangle\,|0\rangle \to \frac{1}{\sqrt{2}}\left(|1\rangle\,|0\rangle + |0\rangle\,|1\rangle\right) \tag{S45}$$

thereby implementing the desired Hadamard gate.

Crucially, the order of braiding operations is determined solely via the topography of domain walls. For instance, a suitable change to the topography in Fig. 1 (right) changes the Hadamard gate to an identity operation. This permits control of the respective quantum operations via optical means.

[1] M. Sigrist and K. Ueda, Rev. Mod. Phys. **63**, 239 (1991).

[2] A. M. Black-Schaffer and C. Honerkamp, J. Phys. Condens. Matter **26**, 423201 (2014).

[3] D. Vollhardt, Rev. Mod. Phys. **56**, 99 (1984).

[4] F. C. Zhang, C. Gros, T. M. Rice, and H. Shiba, Supercond. Sci. Technol. **1**, 36 (1988).

[5] A. Altland and B. Simons, *Condensed Matter Field Theory* (Cambridge University Press, Cambridge, England, 2010).

[6] N. Kopnin, *Theory of Nonequilibrium Superconductivity* (Oxford University Press, New York, 2001).
[7] Y. Nambu, Phys. Rev. **117**, 648 (1960).
[8] B. Lian, X.-Q. Sun, A. Vaezi, X.-L. Qi, and S.-C. Zhang, PNAS **115**, 10938–10942 (2018).
